# Supplementary material for: Graphene: Infrastructure Security Posture Analysis with AI-generated Attack Graphs
Source: arXiv:2312.13119 source file (2024-05-01)
Supplement: Supplementary file 1 [file Hyperparameters.tex]

\section{Hyperparameters}
